# Supplementary material for: Generalized Lazy Search for Robot Motion Planning: Interleaving Search and Edge Evaluation via Event-based Toggles
Source: arXiv:1904.02795 source file (2019-07-22)
Supplement: Supplementary file 4 [file old_results.tex]

\section{Experimental Results}
\subsection{\texttt{Easy} Environment}
%
\begin{figure*}[h]
\centering
  \begin{subfigure}[b]{0.25\textwidth}
    \centering
    \includegraphics[width = \textwidth]{new_figs/square_delta/1_evals}
    \caption{}
    \label{fig:app_3evals}
    \vspace*{1em}
  \end{subfigure}
  \begin{subfigure}[b]{0.25\textwidth}
    \centering
    \includegraphics[width = \textwidth]{new_figs/square_delta/2_evals}
    \caption{}
    \label{fig:app_26evals}
    \vspace*{1em}
  \end{subfigure}
  \begin{subfigure}[b]{0.25\textwidth}
    \centering
    \includegraphics[width = \textwidth]{new_figs/square_delta/3_evals}
    \caption{}
    \label{fig:app_47evals}
    \vspace*{1em}
  \end{subfigure}
%%%%%%%%%%%%%%%%%%%%%%%%%%%%%%%
  \begin{subfigure}[b]{0.25\textwidth}
    \centering
    \includegraphics[width = \textwidth]{new_figs/square_delta/4_evals}
    \caption{}
    \label{fig:app_3evals}
    \vspace*{1em}
  \end{subfigure}
  \begin{subfigure}[b]{0.25\textwidth}
    \centering
    \includegraphics[width = \textwidth]{new_figs/square_delta/5_evals}
    \caption{}
    \label{fig:app_26evals}
    \vspace*{1em}
  \end{subfigure}
  \begin{subfigure}[b]{0.25\textwidth}
    \centering
    \includegraphics[width = \textwidth]{new_figs/square_delta/6_evals}
    \caption{}
    \label{fig:app_47evals}
    \vspace*{1em}
  \end{subfigure}
%%%%%%%%%%%%%%%%%%%%%%%%%%%%%%%
  \begin{subfigure}[b]{0.25\textwidth}
    \centering
    \includegraphics[width = \textwidth]{new_figs/square_delta/7_evals}
    \caption{}
    \label{fig:app_3evals}
    \vspace*{1em}
  \end{subfigure}
  \begin{subfigure}[b]{0.25\textwidth}
    \centering
    \includegraphics[width = \textwidth]{new_figs/square_delta/8_evals}
    \caption{}
    \label{fig:app_26evals}
    \vspace*{1em}
  \end{subfigure}
  \begin{subfigure}[b]{0.25\textwidth}
    \centering
    \includegraphics[width = \textwidth]{new_figs/square_delta/9_evals}
    \caption{}
    \label{fig:app_47evals}
    \vspace*{1em}
  \end{subfigure}
%%%%%%%%%%%%%%%%%%%%%%%%%%%%%%%
  \begin{subfigure}[b]{0.25\textwidth}
    \centering
    \includegraphics[width=\textwidth]{new_figs/square_delta/10_evals}
    \caption{}
    \label{fig:app_3evals}
    \vspace*{1em}
  \end{subfigure}
  \begin{subfigure}[b]{0.25\textwidth}
    \centering
    \includegraphics[width=\textwidth]{new_figs/square_delta/11_evals}
    \caption{}
    \label{fig:app_26evals}
    \vspace*{1em}
  \end{subfigure}
  \begin{subfigure}[b]{0.25\textwidth}
    \centering
    \includegraphics[width=\textwidth]{new_figs/square_delta/12_evals}
    \caption{}
    \label{fig:app_47evals}
    \vspace*{1em}
  \end{subfigure}
%%%%%%%%%%%%%%%%%%%%%%%%%%%%%%%
  \begin{subfigure}[b]{0.25\textwidth}
    \centering
    \includegraphics[width=\textwidth]{new_figs/square_delta/13_evals}
    \caption{}
    \label{fig:app_3evals}
    \vspace*{1em}
  \end{subfigure}
  \begin{subfigure}[b]{0.25\textwidth}
    \centering
    \includegraphics[width=\textwidth]{new_figs/square_delta/14_evals}
    \caption{}
    \label{fig:app_26evals}
    \vspace*{1em}
  \end{subfigure}
  \begin{subfigure}[b]{0.25\textwidth}
    \centering
    \includegraphics[width=\textwidth]{new_figs/square_delta/15_evals}
    \caption{}
    \label{fig:app_47evals}
    \vspace*{1em}
  \end{subfigure}
%%%%%%%%%%%%%%%%%%%%%%%%%%%%%%%
%%%%%%%%%%%%%%%%%%%%%%%%%%%%%%%
\caption{\texttt{Easy}: Number of edge evaluations as a function of $\delta$ for informed search with forward and greedy selectors.}
\label{fig:easy_app_evals}
\end{figure*}


\begin{figure*}[!ht]
\centering
  \begin{subfigure}[b]{0.25\textwidth}
    \centering
    \includegraphics[width = \textwidth]{new_figs/square_delta/1_rewires}
    \caption{}
    \label{fig:app_3rewires}
    \vspace*{1em}
  \end{subfigure}
  \begin{subfigure}[b]{0.25\textwidth}
    \centering
    \includegraphics[width = \textwidth]{new_figs/square_delta/2_rewires}
    \caption{}
    \label{fig:app_26rewires}
    \vspace*{1em}
  \end{subfigure}
  \begin{subfigure}[b]{0.25\textwidth}
    \centering
    \includegraphics[width = \textwidth]{new_figs/square_delta/3_rewires}
    \caption{}
    \label{fig:app_47rewires}
    \vspace*{1em}
  \end{subfigure}
%%%%%%%%%%%%%%%%%%%%%%%%%%%%%%%
  \begin{subfigure}[b]{0.25\textwidth}
    \centering
    \includegraphics[width = \textwidth]{new_figs/square_delta/4_rewires}
    \caption{}
    \label{fig:app_3rewires}
    \vspace*{1em}
  \end{subfigure}
  \begin{subfigure}[b]{0.25\textwidth}
    \centering
    \includegraphics[width = \textwidth]{new_figs/square_delta/5_rewires}
    \caption{}
    \label{fig:app_26rewires}
    \vspace*{1em}
  \end{subfigure}
  \begin{subfigure}[b]{0.25\textwidth}
    \centering
    \includegraphics[width = \textwidth]{new_figs/square_delta/6_rewires}
    \caption{}
    \label{fig:app_47rewires}
    \vspace*{1em}
  \end{subfigure}
%%%%%%%%%%%%%%%%%%%%%%%%%%%%%%%
  \begin{subfigure}[b]{0.25\textwidth}
    \centering
    \includegraphics[width = \textwidth]{new_figs/square_delta/7_rewires}
    \caption{}
    \label{fig:app_3rewires}
    \vspace*{1em}
  \end{subfigure}
  \begin{subfigure}[b]{0.25\textwidth}
    \centering
    \includegraphics[width = \textwidth]{new_figs/square_delta/8_rewires}
    \caption{}
    \label{fig:app_26rewires}
    \vspace*{1em}
  \end{subfigure}
  \begin{subfigure}[b]{0.25\textwidth}
    \centering
    \includegraphics[width = \textwidth]{new_figs/square_delta/9_rewires}
    \caption{}
    \label{fig:app_47rewires}
    \vspace*{1em}
  \end{subfigure}
%%%%%%%%%%%%%%%%%%%%%%%%%%%%%%%
  \begin{subfigure}[b]{0.25\textwidth}
    \centering
    \includegraphics[width=\textwidth]{new_figs/square_delta/10_rewires}
    \caption{}
    \label{fig:app_3rewires}
    \vspace*{1em}
  \end{subfigure}
  \begin{subfigure}[b]{0.25\textwidth}
    \centering
    \includegraphics[width=\textwidth]{new_figs/square_delta/11_rewires}
    \caption{}
    \label{fig:app_26rewires}
    \vspace*{1em}
  \end{subfigure}
  \begin{subfigure}[b]{0.25\textwidth}
    \centering
    \includegraphics[width=\textwidth]{new_figs/square_delta/12_rewires}
    \caption{}
    \label{fig:app_47rewires}
    \vspace*{1em}
  \end{subfigure}
%%%%%%%%%%%%%%%%%%%%%%%%%%%%%%%
  \begin{subfigure}[b]{0.25\textwidth}
    \centering
    \includegraphics[width=\textwidth]{new_figs/square_delta/13_rewires}
    \caption{}
    \label{fig:app_3rewires}
    \vspace*{1em}
  \end{subfigure}
  \begin{subfigure}[b]{0.25\textwidth}
    \centering
    \includegraphics[width=\textwidth]{new_figs/square_delta/14_rewires}
    \caption{}
    \label{fig:app_26rewires}
    \vspace*{1em}
  \end{subfigure}
  \begin{subfigure}[b]{0.25\textwidth}
    \centering
    \includegraphics[width=\textwidth]{new_figs/square_delta/15_rewires}
    \caption{}
    \label{fig:app_47rewires}
    \vspace*{1em}
  \end{subfigure}
%%%%%%%%%%%%%%%%%%%%%%%%%%%%%%%
%%%%%%%%%%%%%%%%%%%%%%%%%%%%%%%
\caption{\texttt{Easy}: Number of edge rewires as a function of $\delta$ for informed search with forward and greedy selectors.}
\label{fig:easy_app_rewires}
\end{figure*}



\subsection{\texttt{Hard} Environment}


\begin{figure*}[!ht]
\centering
  \begin{subfigure}[b]{0.25\textwidth}
    \centering
    \includegraphics[width = \textwidth]{new_figs/two_wall_delta/3_evals}
    \caption{}
    \label{fig:app_3evals}
    \vspace*{1em}
  \end{subfigure}
  \begin{subfigure}[b]{0.25\textwidth}
    \centering
    \includegraphics[width = \textwidth]{new_figs/two_wall_delta/26_evals}
    \caption{}
    \label{fig:app_26evals}
    \vspace*{1em}
  \end{subfigure}
  \begin{subfigure}[b]{0.25\textwidth}
    \centering
    \includegraphics[width = \textwidth]{new_figs/two_wall_delta/47_evals}
    \caption{}
    \label{fig:app_47evals}
    \vspace*{1em}
  \end{subfigure}
%%%%%%%%%%%%%%%%%%%%%%%%%%%%%%%
  \begin{subfigure}[b]{0.25\textwidth}
    \centering
    \includegraphics[width = \textwidth]{new_figs/two_wall_delta/92_evals}
    \caption{}
    \label{fig:app_3evals}
    \vspace*{1em}
  \end{subfigure}
  \begin{subfigure}[b]{0.25\textwidth}
    \centering
    \includegraphics[width = \textwidth]{new_figs/two_wall_delta/108_evals}
    \caption{}
    \label{fig:app_26evals}
    \vspace*{1em}
  \end{subfigure}
  \begin{subfigure}[b]{0.25\textwidth}
    \centering
    \includegraphics[width = \textwidth]{new_figs/two_wall_delta/117_evals}
    \caption{}
    \label{fig:app_47evals}
    \vspace*{1em}
  \end{subfigure}
%%%%%%%%%%%%%%%%%%%%%%%%%%%%%%%
  \begin{subfigure}[b]{0.25\textwidth}
    \centering
    \includegraphics[width = \textwidth]{new_figs/two_wall_delta/130_evals}
    \caption{}
    \label{fig:app_3evals}
    \vspace*{1em}
  \end{subfigure}
  \begin{subfigure}[b]{0.25\textwidth}
    \centering
    \includegraphics[width = \textwidth]{new_figs/two_wall_delta/149_evals}
    \caption{}
    \label{fig:app_26evals}
    \vspace*{1em}
  \end{subfigure}
  \begin{subfigure}[b]{0.25\textwidth}
    \centering
    \includegraphics[width = \textwidth]{new_figs/two_wall_delta/163_evals}
    \caption{}
    \label{fig:app_47evals}
    \vspace*{1em}
  \end{subfigure}
%%%%%%%%%%%%%%%%%%%%%%%%%%%%%%%
  \begin{subfigure}[b]{0.25\textwidth}
    \centering
    \includegraphics[width=\textwidth]{new_figs/two_wall_delta/171_evals}
    \caption{}
    \label{fig:app_3evals}
    \vspace*{1em}
  \end{subfigure}
  \begin{subfigure}[b]{0.25\textwidth}
    \centering
    \includegraphics[width=\textwidth]{new_figs/two_wall_delta/176_evals}
    \caption{}
    \label{fig:app_26evals}
    \vspace*{1em}
  \end{subfigure}
  \begin{subfigure}[b]{0.25\textwidth}
    \centering
    \includegraphics[width=\textwidth]{new_figs/two_wall_delta/194_evals}
    \caption{}
    \label{fig:app_47evals}
    \vspace*{1em}
  \end{subfigure}
%%%%%%%%%%%%%%%%%%%%%%%%%%%%%%%
  \begin{subfigure}[b]{0.25\textwidth}
    \centering
    \includegraphics[width=\textwidth]{new_figs/two_wall_delta/209_evals}
    \caption{}
    \label{fig:app_3evals}
    \vspace*{1em}
  \end{subfigure}
  \begin{subfigure}[b]{0.25\textwidth}
    \centering
    \includegraphics[width=\textwidth]{new_figs/two_wall_delta/277_evals}
    \caption{}
    \label{fig:app_26evals}
    \vspace*{1em}
  \end{subfigure}
  \begin{subfigure}[b]{0.25\textwidth}
    \centering
    \includegraphics[width=\textwidth]{new_figs/two_wall_delta/283_evals}
    \caption{}
    \label{fig:app_47evals}
    \vspace*{1em}
  \end{subfigure}
%%%%%%%%%%%%%%%%%%%%%%%%%%%%%%%
%%%%%%%%%%%%%%%%%%%%%%%%%%%%%%%
\caption{\texttt{Hard}: Number of edge evaluations as a function of $\delta$ for informed search with forward and greedy selectors.}
\label{fig:hard_app_evals}
\end{figure*}


\begin{figure*}[!ht]
\centering
  \begin{subfigure}[b]{0.25\textwidth}
    \centering
    \includegraphics[width = \textwidth]{new_figs/two_wall_delta/3_rewires}
    \caption{}
    \label{fig:app_3rewires}
    \vspace*{1em}
  \end{subfigure}
  \begin{subfigure}[b]{0.25\textwidth}
    \centering
    \includegraphics[width = \textwidth]{new_figs/two_wall_delta/26_rewires}
    \caption{}
    \label{fig:app_26rewires}
    \vspace*{1em}
  \end{subfigure}
  \begin{subfigure}[b]{0.25\textwidth}
    \centering
    \includegraphics[width = \textwidth]{new_figs/two_wall_delta/47_rewires}
    \caption{}
    \label{fig:app_47rewires}
    \vspace*{1em}
  \end{subfigure}
%%%%%%%%%%%%%%%%%%%%%%%%%%%%%%%
  \begin{subfigure}[b]{0.25\textwidth}
    \centering
    \includegraphics[width = \textwidth]{new_figs/two_wall_delta/92_rewires}
    \caption{}
    \label{fig:app_3rewires}
    \vspace*{1em}
  \end{subfigure}
  \begin{subfigure}[b]{0.25\textwidth}
    \centering
    \includegraphics[width = \textwidth]{new_figs/two_wall_delta/108_rewires}
    \caption{}
    \label{fig:app_26rewires}
    \vspace*{1em}
  \end{subfigure}
  \begin{subfigure}[b]{0.25\textwidth}
    \centering
    \includegraphics[width = \textwidth]{new_figs/two_wall_delta/117_rewires}
    \caption{}
    \label{fig:app_47rewires}
    \vspace*{1em}
  \end{subfigure}
%%%%%%%%%%%%%%%%%%%%%%%%%%%%%%%
  \begin{subfigure}[b]{0.25\textwidth}
    \centering
    \includegraphics[width = \textwidth]{new_figs/two_wall_delta/130_rewires}
    \caption{}
    \label{fig:app_3rewires}
    \vspace*{1em}
  \end{subfigure}
  \begin{subfigure}[b]{0.25\textwidth}
    \centering
    \includegraphics[width = \textwidth]{new_figs/two_wall_delta/149_rewires}
    \caption{}
    \label{fig:app_26rewires}
    \vspace*{1em}
  \end{subfigure}
  \begin{subfigure}[b]{0.25\textwidth}
    \centering
    \includegraphics[width = \textwidth]{new_figs/two_wall_delta/163_rewires}
    \caption{}
    \label{fig:app_47rewires}
    \vspace*{1em}
  \end{subfigure}
%%%%%%%%%%%%%%%%%%%%%%%%%%%%%%%
  \begin{subfigure}[b]{0.25\textwidth}
    \centering
    \includegraphics[width=\textwidth]{new_figs/two_wall_delta/171_rewires}
    \caption{}
    \label{fig:app_3rewires}
    \vspace*{1em}
  \end{subfigure}
  \begin{subfigure}[b]{0.25\textwidth}
    \centering
    \includegraphics[width=\textwidth]{new_figs/two_wall_delta/176_rewires}
    \caption{}
    \label{fig:app_26rewires}
    \vspace*{1em}
  \end{subfigure}
  \begin{subfigure}[b]{0.25\textwidth}
    \centering
    \includegraphics[width=\textwidth]{new_figs/two_wall_delta/194_rewires}
    \caption{}
    \label{fig:app_47rewires}
    \vspace*{1em}
  \end{subfigure}
%%%%%%%%%%%%%%%%%%%%%%%%%%%%%%%
  \begin{subfigure}[b]{0.25\textwidth}
    \centering
    \includegraphics[width=\textwidth]{new_figs/two_wall_delta/209_rewires}
    \caption{}
    \label{fig:app_3rewires}
    \vspace*{1em}
  \end{subfigure}
  \begin{subfigure}[b]{0.25\textwidth}
    \centering
    \includegraphics[width=\textwidth]{new_figs/two_wall_delta/277_rewires}
    \caption{}
    \label{fig:app_26rewires}
    \vspace*{1em}
  \end{subfigure}
  \begin{subfigure}[b]{0.25\textwidth}
    \centering
    \includegraphics[width=\textwidth]{new_figs/two_wall_delta/283_rewires}
    \caption{}
    \label{fig:app_47rewires}
    \vspace*{1em}
  \end{subfigure}
%%%%%%%%%%%%%%%%%%%%%%%%%%%%%%%
\caption{\texttt{Hard}: Number of edge rewires as a function of $\delta$ for informed search with forward and greedy selectors.}
\label{fig:hard_app_rewires}
\end{figure*}
